# Supplementary material for: Composition Effects on Ni/Al Reactive Multilayers: A Comprehensive Study of Mechanical Properties, Reaction Dynamics and Phase Evolution
Source: arXiv:2502.02333 ancillary file (2025-02-04)
Supplement: Supplementary file 1 [file supplementary_material.pdf]

**Supplementary Material: Composition Effects on Ni/Al Reactive Multilayers: A Comprehensive Study of Mechanical Properties, Reaction Dynamics and Phase Evolution**

N. Toncich,<sup>1</sup> F. Schwarz,<sup>1</sup> R.A. Gallivan,<sup>1</sup> J. Gillon,<sup>1</sup> and R. Spolenak<sup>1</sup>

*Laboratory for Nanometallurgy, Department of Materials, ETH Zurich*

(\*Electronic mail: nensi.toncich@mat.ethz.ch)

## I. AS-DEPOSITED ANALYSIS

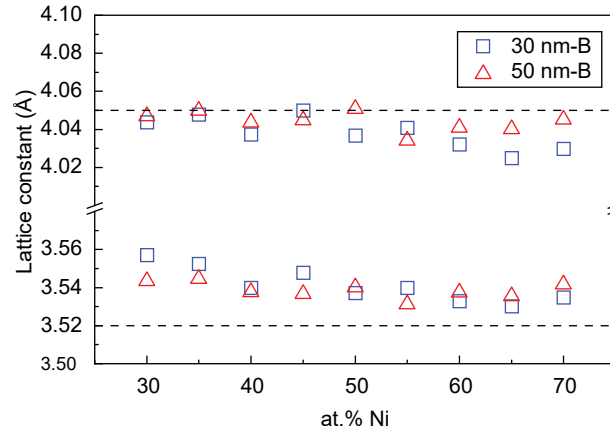

Figure 1. Lattice spacing in Ni and Al layers for the 30 nm and 50 nm-B systems. The lattice spacing is determined from the predominant peaks in the XRD diffraction pattern: Ni(111) and Al(111). Dashed lines indicate the lattice constants of unstressed Ni<sup>1</sup> and Al<sup>2</sup>. A slight increase in the Ni lattice constant is observed in Al-rich compositions, whereas a decrease in the Al lattice constant occurs in Ni-rich compositions. This effect is more prominent in the thinner bilayer systems and it may result from stress associated with the layer thickness or the formation of a metastable solid solution.

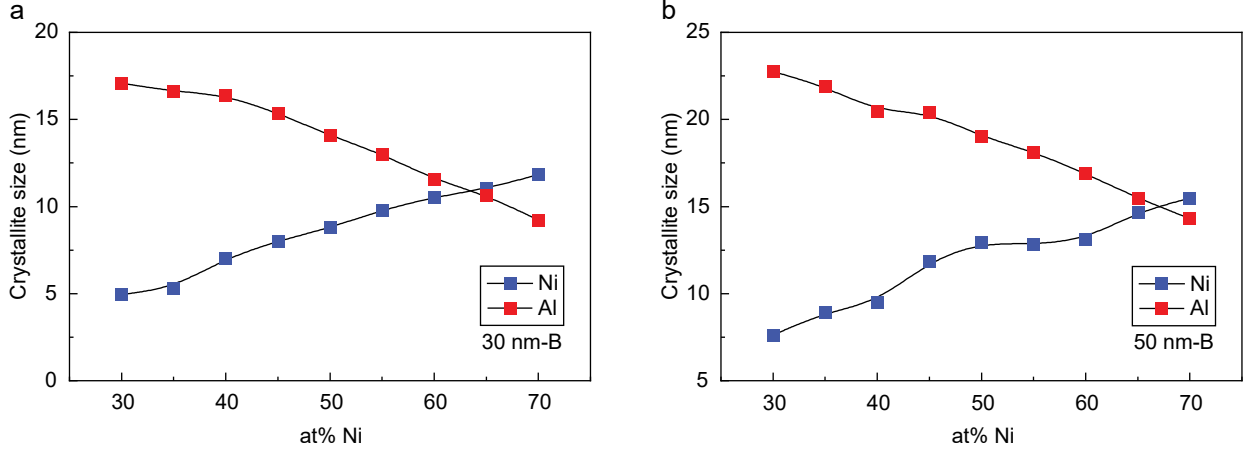

SFigure 2. Crystallite size of the Ni and Al layer in (a) 30 nm-B samples and (b) 50 nm-B samples. The Ni(111) and Al(111) peaks were selected for the determination of the crystallite size using the Scherrer equation. All films exhibit nanoscale crystallites, with size variations primarily dependent on the individual layer thickness across different sample stoichiometries. A plateau in crystallite size is observed for compositions ranging from 50 to 60 at.% Ni in 50 nm-B systems, suggesting that the grain size is controlled by layer thickness up to 20 nm.

## II. AFTER IGNITION STUDY

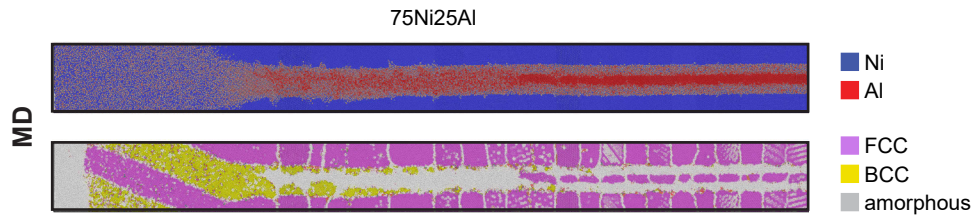

SFigure 3. Simulated microstructures of ignited 75Ni25Al system with a bilayer thickness of 15 nm and a 2 nm-thick intermixed layer, observed 6 ns after ignition. The top figure depicts atom types, with Ni shown in blue and Al in red, while the bottom figure represents crystal structures, with FCC in purple, BCC in yellow, and amorphous regions in grey. Behind the reaction front, both FCC and BCC phases are observed. The BCC phase is likely B2-AlNi, while the FCC is likely L1-Ni<sub>3</sub>Al, with a Ni excess<sup>3</sup>.

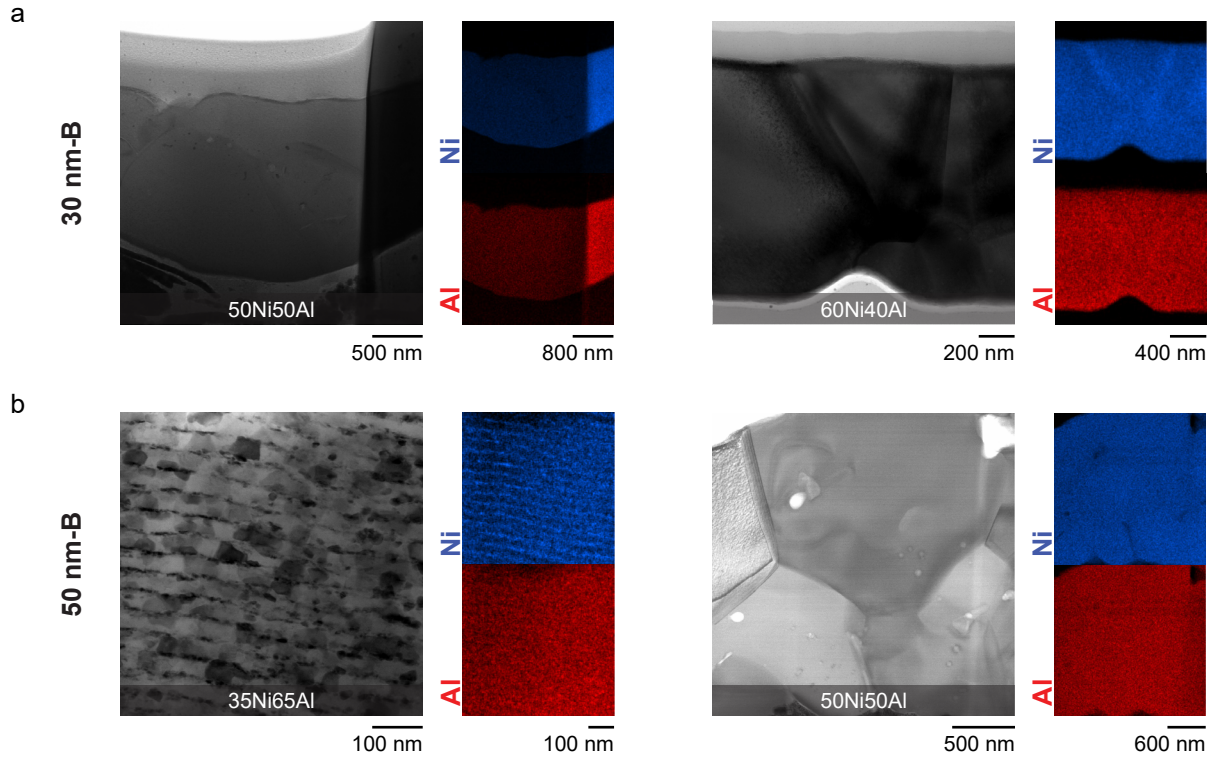

Figure 4. Experimental microstructures of ignited Ni/Al systems. (a) BF-STEM images and EDX composition maps of the 50Ni50Al (left) and 60Ni40Al (right) systems with 30 nm-B, showing comparable grain sizes of the B2-NiAl phase in both samples. (b) BF-STEM images and EDX composition maps of the 35Ni65Al (left) and 50Ni50Al (right) systems with 50 nm-B. The 35Ni65Al sample reveals a quenched, partially transformed region with residual Ni layers, indicating incomplete formation of the intermetallic phase. The 50Ni50Al sample shows fully formed grains corresponding to the B2-NiAl phase.



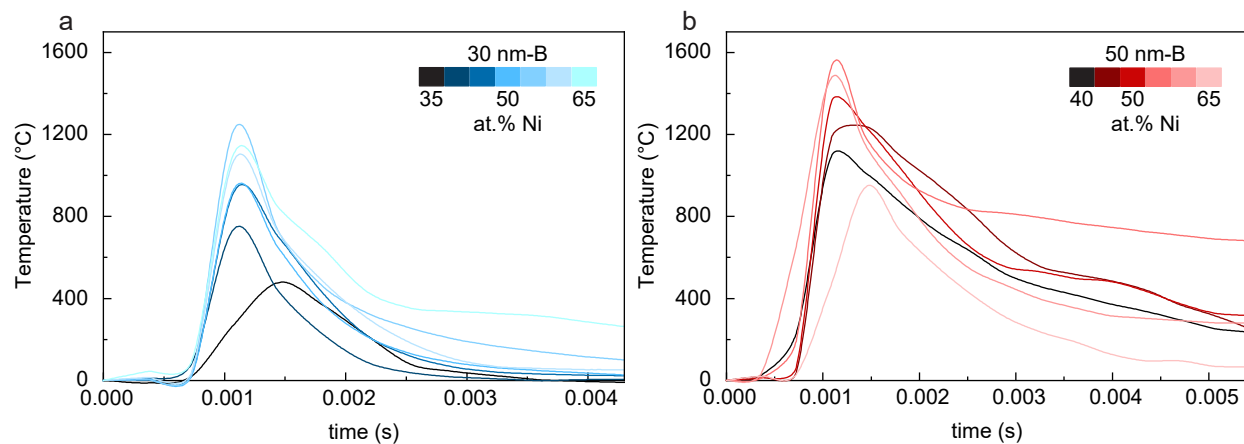

Figure 5. Temperature–time curves obtained using a high-speed infrared camera during the self-sustained reaction of Ni/Al RMs with different stoichiometries and bilayer thicknesses of (a) 30 nm and (b) 50 nm. The maximum temperatures achieved vary with Ni/Al stoichiometry. Following the progression of the reaction front, the temperatures rapidly return to ambient within milliseconds.

## REFERENCES

- <sup>1</sup>P. Du, P. Wu, and C. Cai, “Mechanistic insight into the facet-dependent adsorption of methanol on a Pt<sub>3</sub>Ni nanocatalyst,” *The Journal of Physical Chemistry C* **119**, 18352–18363 (2015).
- <sup>2</sup>F. Tang, X. Che, W. Lu, G. Chen, Y. Xie, and W. Yu, “Surface structure and solidification morphology of aluminum nanoclusters,” *Physica B: Condensed Matter* **404**, 2489–2494 (2009).
- <sup>3</sup>F. Schwarz, *Using molecular dynamics simulations to better understand and predict the behavior of reactive multilayers*, Ph.D. thesis, ETH Zurich (2023).
